# Supplementary material for: Differential Operator Representation of sl (2, R) as Modules over Univariate and Bivariate Hermite Polynomials
Source: arXiv:2309.03916 source file (2023-09-12)
Supplement: Supplementary file 1 [file appendix.tex]

\section{Appendix }

\textup{For validation of equation (93), We calculated the $\lim_{t\to 0} g(x,t)$ by online calculator \href{https://keisan.casio.com/exec/system/1180573447}{keisan}. Calculations of equation (90) for $z=1200$ and $z=2000$ while $t$ is small, result in 0.994 and 0.997 for $g(x,t)$  respectively. this verifies the limit in equation (93).
